# Supplementary material for: CCDD: A Tractable Representation for Model Counting and Uniform Sampling
Source: arXiv:2202.10025 source file (2022-02-21)
Supplement: Supplementary file 1 [file Appendix.tex]

\newpage
\appendix
\section{Appendix}\label{stylefiles}
\subsection{Errata} In preparation of the artifact, we discovered a minor bug in a script whose output was used to generate Table 1, Table 2, and Figure 3. The bug only affected the solving time statistics 
% Thankfully, the bug only affected the solving time statistics
of ADDMC for the instances that ADDMC solved.
 We remark that these statistics do not have
any impact on the conclusion of the paper or interpretation of the results, since ADDMC
solved the least instances in our experiments. 
While there is no significant impact, we present an update of the data in
the experimental section of the paper 
% We updated some data in the section of experiments 
in this appendix:

\begin{itemize}
	\item We revised Figure \ref{fig:counting:time} as Figure \ref{fig:counting2:time}. We remark that we only modified the curve of ADDMC. Again, note that ADDMC solves the least number of instances. 
	\item The three numbers in the ADDMC column of Table 2 should be 0.3, 0.7, and 0.1 from top to bottom, respectively.
	\item The first two sentences in the last paragraph of Section 5 should be as follows: \\[1mm]
		We analyze the running time for individual instances by omitting the easy instances (solved by at least five tools in under 2 seconds) and hard instances (not solved by any tool). 
	\ExactMC{}
	performed the best on 39.5\% instances, while Ganak, c2d,
	miniC2D, D4, and ADDMC performed the best on 22.3\%,
	2.5\%, 3.9\%, 16.1\%, and 15.7\%, respectively.
\end{itemize}

\begin{figure}[htb]
	\centering
	\includegraphics[width = \linewidth]{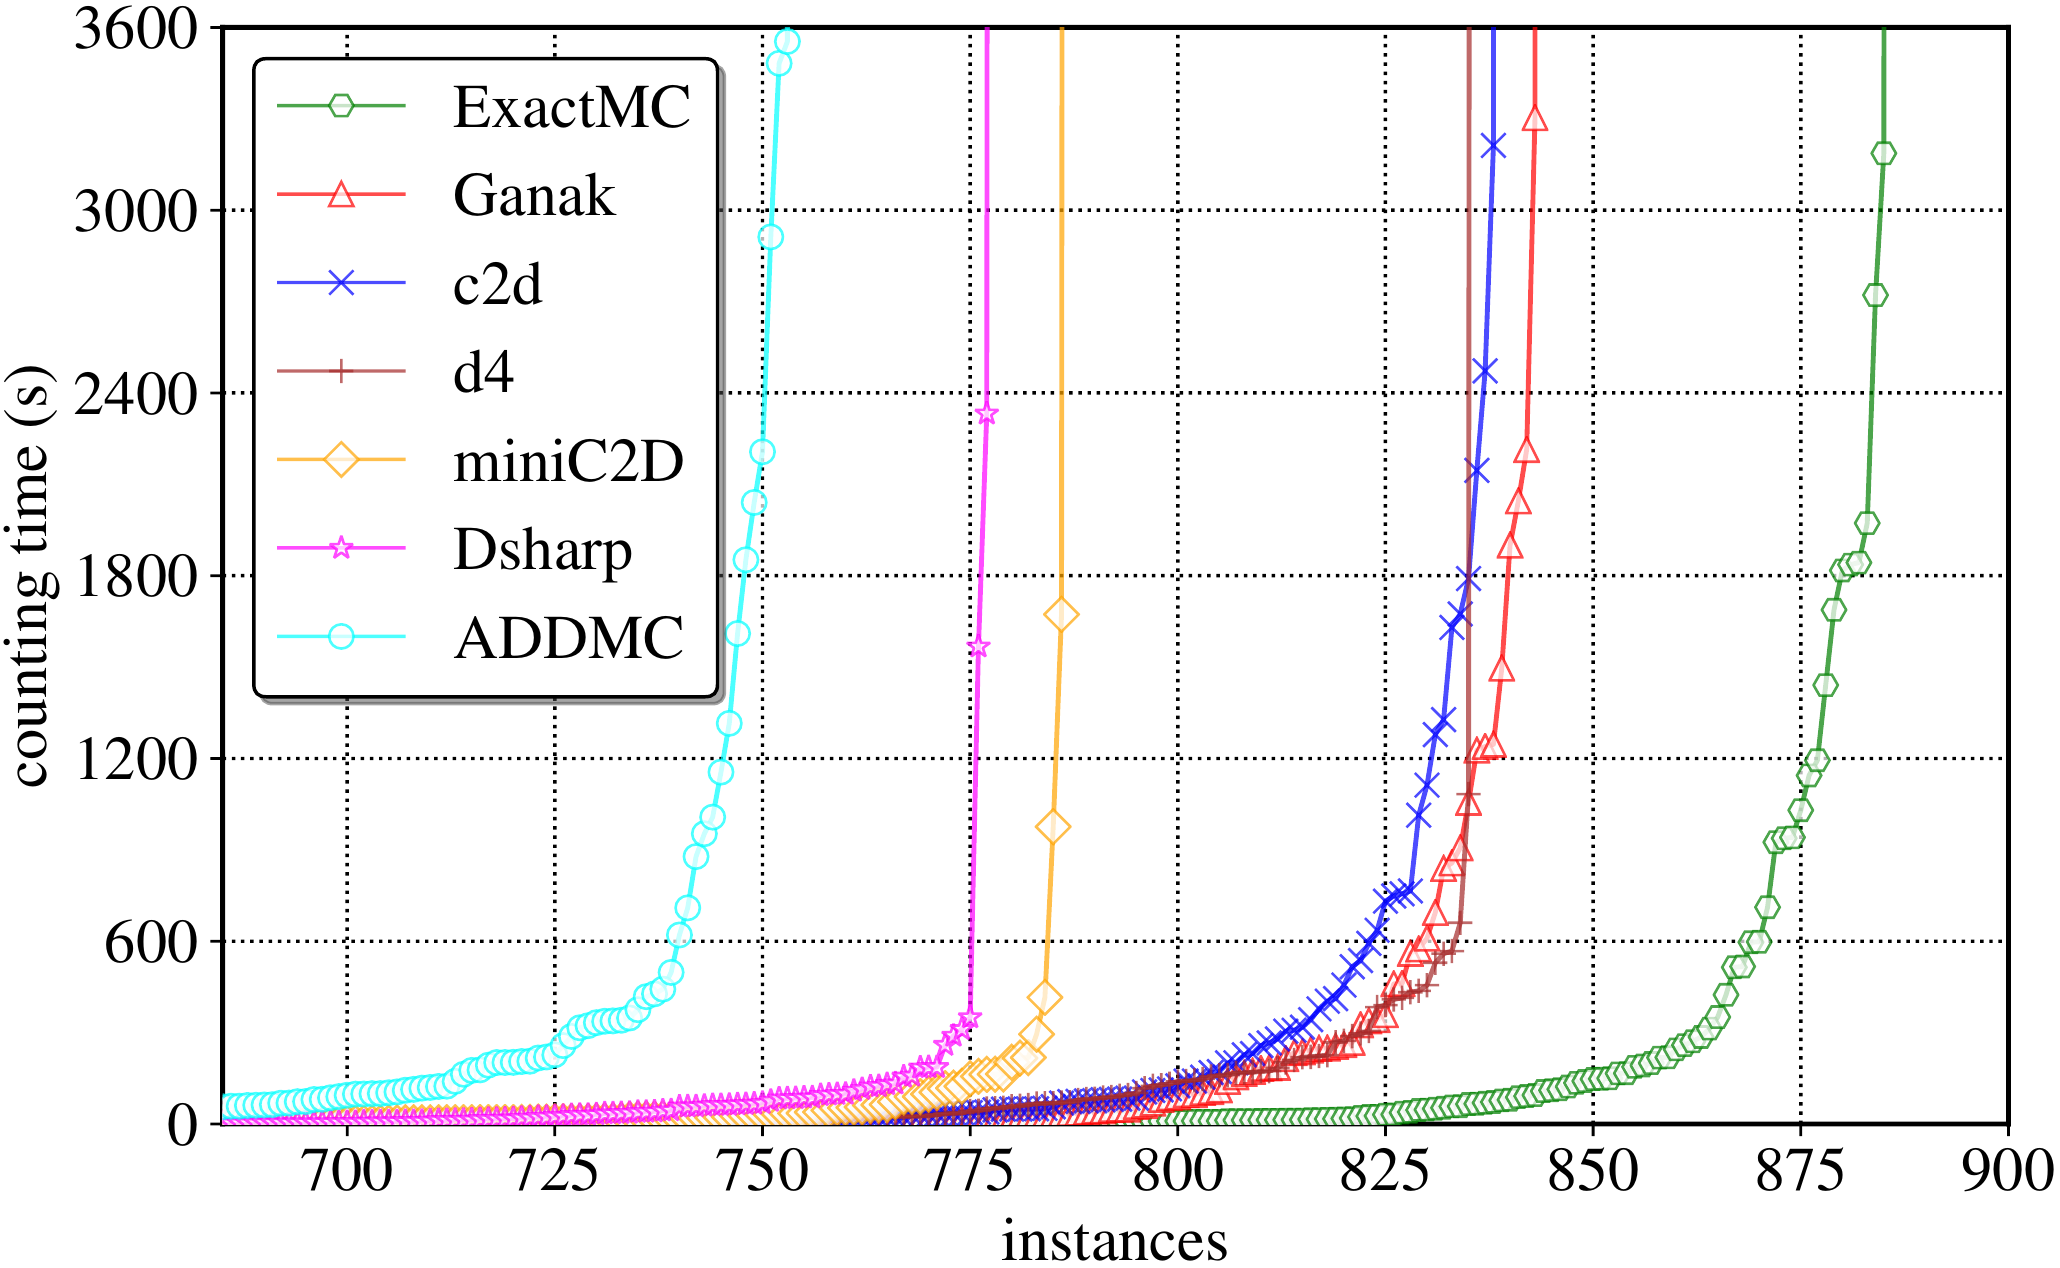}
	\caption{Cactus plot comparing the solving time of different counters. (Best viewed in color)}\label{fig:counting2:time}
\end{figure}

\subsection{Proof of Theorem~\ref{thm:compl}}
\completeness*

\begin{proof}
If we remove the case (ii) in Definition \ref{def:RCDD}, the \CDD{} is a \DecDNNF{} formula.
In other words, \DecDNNF{} is a subset of \Ctwo{}. Since \CNF{} is complete, and each \CNF{} formula can be compiled into \DecDNNF{} \cite{Oztok:Darwiche:14}, we obtain the completeness of \Ctwo{}:	
\end{proof}

\subsection{Detailed Experimental Results}
Finally, we present the detailed results of Ganak, c2d, miniC2D, D4, ADDMC, and \ExactMC{} in Table \ref{tab:detailed-results}.

\onecolumn
\begin{center}
	\footnotesize
	% [inline block 0: 1 envs, 102679 chars -> data_tex | \begin{longtable}{|p{8cm}|p{1cm}|p{1cm}|p{1cm}|p{1cm}|p{1cm}|p{1cm}|} 		\caption{Detailed benchmark results. Some specia...]

\end{center}
